# Supplementary material for: Electronic and Optical Excitations in van der Waals Materials from a Non-Empirical Wannier-Localized Optimally-Tuned Screened Range-Separated Hybrid Functional
Source: arXiv:2405.00643 ancillary file (2024-05-01)
Supplement: Supplementary file 1 [file SI.pdf]

## Supporting Information

# Electronic and Optical Excitations in van der Waals Materials from a Non-Empirical Wannier-Localized Optimally-Tuned Screened Range-Separated Hybrid Functional

María Camarasa-Gómez,<sup>1</sup> Stephen E. Gant,<sup>2,3</sup> Guy Ohad,<sup>1</sup> Jeffrey  
B. Neaton,<sup>2,3,4</sup> Ashwin Ramasubramaniam,<sup>5,6</sup> and Leeor Kronik<sup>1,\*</sup>

<sup>1</sup>*Department of Molecular Chemistry and Materials Science,  
Weizmann Institute of Science, Rehovoth 7610001, Israel*

<sup>2</sup>*Department of Physics, University of California, Berkeley, CA 94720, USA*

<sup>3</sup>*Materials Sciences Division, Lawrence Berkeley  
National Laboratory, Berkeley, CA 94720, USA*

<sup>4</sup>*Kavli Energy NanoSciences Institute at Berkeley,  
University of California, Berkeley, CA 94720, USA*

<sup>5</sup>*Department of Mechanical and Industrial Engineering,  
University of Massachusetts Amherst, Amherst MA 01003, USA*

<sup>6</sup>*Materials Science and Engineering Graduate Program,  
University of Massachusetts, Amherst, Amherst MA 01003, USA*

## CONTENTS

|                                             |    |
|---------------------------------------------|----|
| I. Non-empirical WOT-SRSH Functional method | 3  |
| II. Computational details                   | 6  |
| A. General                                  | 6  |
| B. Image-charge corrections                 | 7  |
| C. Band Gap ZPR Computational Details       | 7  |
| D. Atomic Geometries                        | 10 |
| III. Parameters and numerical data          | 13 |
| References                                  | 14 |

## I. NON-EMPIRICAL WOT-SRSH FUNCTIONAL METHOD

Figures S1 and S2 in the following pages demonstrate the selection of optimal parameters for black phosphorous and molybdenum disulphide, respectively, using the non-empirical WOT-SRSH method. They are the equivalent of Figure 1 in the main text, where the same demonstration was given for h-BN.

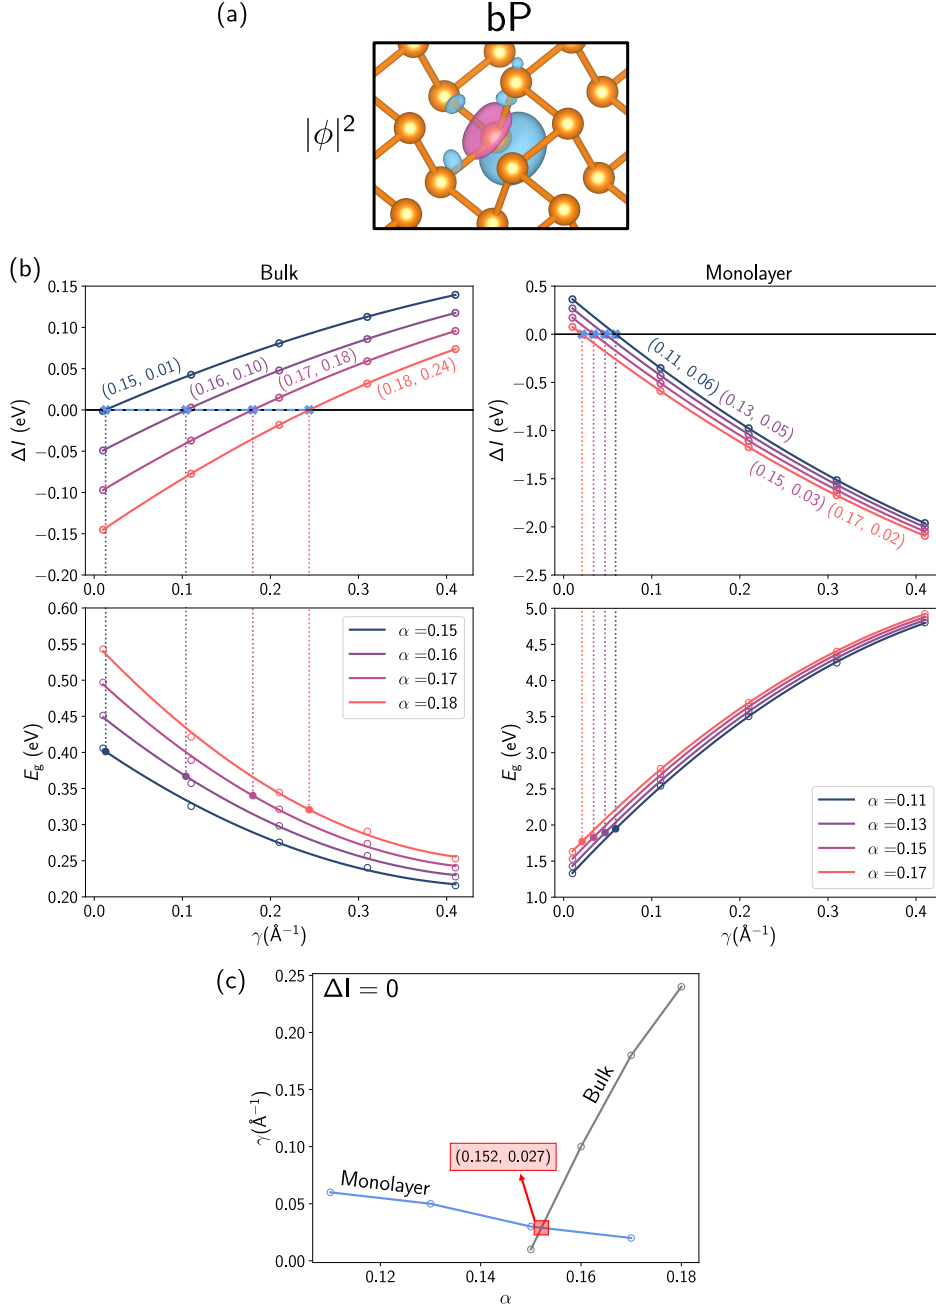

**Fig. S1:** Demonstration of the non-empirical WOT-SRSH method, as applied to black phosphorus (bP): (a) highest-expectation-value occupied maximally-localized Wannier function; (b) The IP ansatz target function,  $\Delta I$  (top) and the fundamental band gap,  $E_g$ , at the  $K$ -point (bottom), for both bulk ( $\epsilon_\infty$  of the solid, left) and monolayer ( $\epsilon_\infty = 1$ , right), as a function of the range-separation parameter,  $\gamma$ , for different values of the fraction of short-range exact exchange,  $\alpha$ . Circles indicated computed data points and the lines are a guide to the eye. Closed circles have been obtained from  $(\alpha, \gamma)$  pairs that obey the IP ansatz, with the parameter values shown; (c) IP ansatz fulfillment ( $\Delta I = 0$ ) curves in the  $(\alpha, \gamma)$  plane for monolayer and bulk, with their point of intersection,  $(\alpha^*, \gamma^*)$ , obeying the IP ansatz for both phases simultaneously and used for predictive calculations.

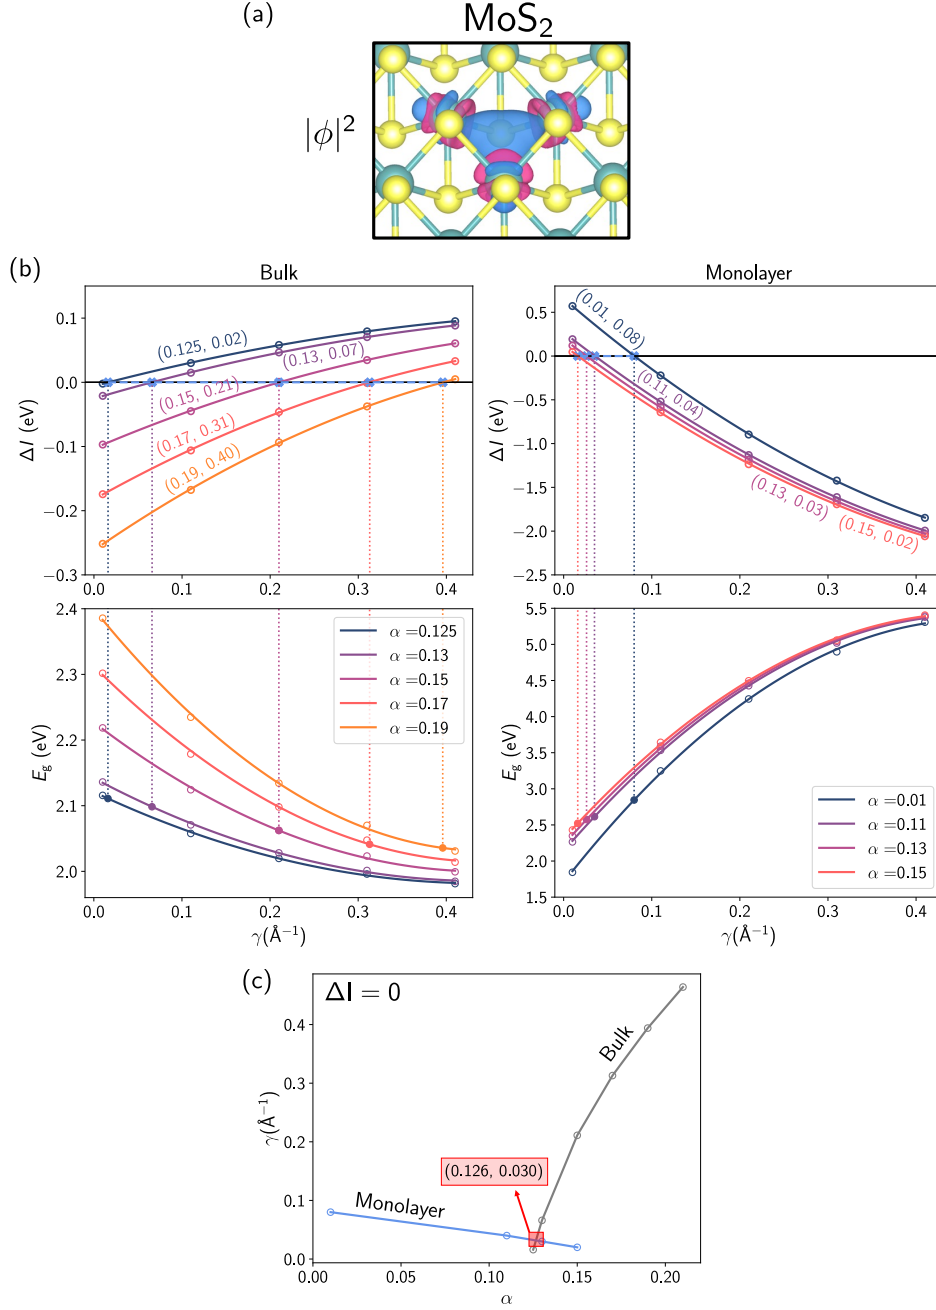

**Fig. S2:** Demonstration of the non-empirical WOT-SRSH method, as applied to  $\text{MoS}_2$ : (a) highest-expectation-value occupied maximally-localized Wannier function; (b) The IP ansatz target function,  $\Delta I$  (top) and the fundamental band gap,  $E_g$ , at the  $K$ -point (bottom), for both bulk ( $\epsilon_\infty$  of the solid, left) and monolayer ( $\epsilon_\infty = 1$ , right), as a function of the range-separation parameter,  $\gamma$ , for different values of the fraction of short-range exact exchange,  $\alpha$ . Circles indicated computed data points and the lines are a guide to the eye. Closed circles have been obtained from  $(\alpha, \gamma)$  pairs that obey the IP ansatz, with the parameter values shown; (c) IP ansatz fulfillment ( $\Delta I = 0$ ) curves in the  $(\alpha, \gamma)$  plane for monolayer and bulk, with their point of intersection,  $(\alpha^*, \gamma^*)$ , obeying the IP ansatz for both phases simultaneously and used for predictive calculations.

## II. COMPUTATIONAL DETAILS

### A. General

All calculations presented in this study were performed using the Vienna *Ab Initio* Simulation Package (VASP)<sup>1,2</sup>, with the exception of the band-gap zero-point renormalization (ZPR) calculations, described separately below. The GW version of the projector-augmented-wave (PAW) pseudopotentials<sup>3,4</sup>, provided with VASP, were utilized to treat core electrons. For molybdenum disulfide (MoS<sub>2</sub>) and hexagonal-boron nitride (h-BN), PAWs based on the local density approximation (LDA)<sup>5,6</sup> were employed, with energy cutoffs set at 500 eV and 550 eV, respectively. For black phosphorus (bP), PAWs based on the Perdew-Burke-Ernzerhof (PBE) functional were employed, with energy cutoffs set at 400 eV for monolayers and 450 eV for bulk, respectively. The electronic configurations of the valence electrons are as follows:  $4s^2 4p^6 5s^1 4d^5$  for Mo,  $3s^2 3p^4$  for S,  $2s^2 2p^1$  for B,  $2s^2 2p^3$  for N, and  $3s^2 3p^3$  for P. Semilocal contributions to electron exchange and correlation in the SRSW were computed within the LDA for MoS<sub>2</sub> and h-BN, and with PBE for bP, in accordance with the PAW pseudopotentials. For the removal of charge from a Wannier function within a constrained SRSW calculation, the Lagrange multiplier that enforces the removal of charge<sup>7</sup> was set to 300 eV. A spin-orbit coupling (SOC) was applied for calculations of monolayer MoS<sub>2</sub>. Detailed information regarding the atomic coordinates and lattice vectors of the unit cells used in this work can be found in Section II D, and from Refs. 8 and 9 and references therein.

Electronic band structures for all materials were calculated utilizing a Wannier interpolation scheme implemented in Wannier90<sup>10</sup> and optical absorption spectra were calculated (within the Tamm-Dancoff approximation) using the time-dependent hybrid-DFT and GW-BSE implementation in VASP. Further computational settings have been provided in Ref. 9. Gaussian broadening of 100 meV was applied to the optical absorption spectra to facilitate comparison with experiment. Macroscopic dielectric constants of MoS<sub>2</sub> and h-BN were calculated using the Random Phase Approximation (RPA)<sup>11</sup>; for bP, which required the use of the HSE06 functional (as noted in the main text), the dielectric constants were calculated via the response to finite external electric fields<sup>12,13</sup>.

## B. Image-charge corrections

As explained in the main text, the ionization potential ansatz<sup>7</sup> that we seek to satisfy in order to tune the SRSB parameters non-empirically is given by

$$\Delta I^\gamma = E_{\text{constr}}^\gamma[\phi](N-1) - E^\gamma(N) + \langle \phi | \hat{H}_{\text{SRSB}}^\gamma | \phi \rangle = 0, \quad (\text{S1})$$

where  $E_{\text{constr}}^\gamma[\phi](N-1)$  is the total energy (calculated via a constrained minimization procedure<sup>7</sup>) of the system with one electron subtracted from the highest occupied maximally-localized Wannier function,  $\phi$  (Figure 1, panel (a)),  $E^\gamma(N)$  is the total energy of the neutral  $N$ -electron system, and  $\langle \phi | \hat{H}_{\text{SRSB}}^\gamma | \phi \rangle$  is the expectation value of the SRSB Hamiltonian  $\hat{H}_{\text{SRSB}}^\gamma$ . As periodic boundary conditions are employed in this work, calculating the energy of the  $(N-1)$ -electron system requires correcting for spurious image-charge interactions. For bulk phases, these corrections are accomplished using anisotropic Makov-Payne image-charge corrections,<sup>14–17</sup> similar to Refs. 7, 18, and 19.

For monolayers, the presence of vacuum in the computational supercell requires a rescaling of the components of the high-frequency dielectric tensor, required as part of the image-charge correction procedure. The in-plane components,  $\epsilon_{xx}$  and  $\epsilon_{yy}$ , are not affected by this rescaling and remain at their bulk phase values<sup>20</sup> whereas the out-of-plane component is rescaled as<sup>21</sup>

$$\epsilon'_{zz} = \frac{t}{L_z} \epsilon_{zz} + \frac{L_z - t}{L_z} \epsilon_0, \quad (\text{S2})$$

where  $t$  is the thickness of the monolayer, which we take to be the interlayer distance,  $L_z$  is supercell vector along the vacuum direction, and  $\epsilon_0 = 1.0$  for vacuum. As a test, we have checked that our values of the rescaled dielectric tensor for monolayer MoS<sub>2</sub> ( $\epsilon'_{xx} = \epsilon'_{yy} = 14.96$ ;  $\epsilon'_{zz} = 2.08$ ) agree with those provided in Ref. 21 ( $\epsilon'_{xx} = \epsilon'_{yy} = 15$ ;  $\epsilon'_{zz} = 2$ ).

## C. Band Gap ZPR Computational Details

Calculations for the ZPR of the fundamental band gap in hBN were carried out in Quantum Espresso<sup>22,23</sup> with the PBE functional<sup>24</sup> using optimized norm-conserving Vanderbilt pseudopotentials<sup>25</sup> from the PseudoDojo repository<sup>26</sup>. Phonon and electron-phonon calculations were set up to run in Quantum Espresso using the soon-to-be-released Caesar code

managed by the Monserrat group at Cambridge, using methods outlined in Refs. 27 and 28. Phonon dispersions for hBN (bulk and monolayer) are computed within the harmonic approximation via the finite difference approaches outlined in Refs. 28 and 29. In the monolayer, the dynamical matrix is solved on both a  $6 \times 6 \times 1$   $q$ -grid and a  $9 \times 9 \times 1$   $q$ -grid, with both yielding very similar results. In the bulk phase, we use  $3 \times 3 \times 1$  and  $6 \times 6 \times 2$   $q$ -grids, finding the use of a  $6 \times 6 \times 2$  grid to have a particularly appreciable impact on ZPR calculations, despite the fact that the resulting phonon dispersions appear quite similar. The zero temperature ZPR of the fundamental gap is then calculated via the Monte Carlo method described in Refs. 27 and 28. In short, for each phase and grid size, a number of corresponding supercells containing a random sampling of displacement configurations, obtained from the previously computed phonon dispersions, are generated. By solving for the Kohn-Sham eigensystem in each configuration, the effects of ZPR on both the valence band maximum and conduction band minimum can be extracted as the means of each distribution of eigenvalues, allowing for the renormalization of the fundamental gap to then be computed. Because this is a statistical approach, the error in the computed ZPR can also be estimated as the standard deviation in the mean of each eigenvalue distribution as reported in Table I. While this approach is expected to capture some level of anharmonic response in the electronic states,<sup>27,28</sup> the ZPR values reported here are still likely to be underestimated, due to the lack of inclusion of non-adiabatic effects.<sup>30</sup> Finally, we emphasize that these corrections are technically for the fundamental gap and not the lowest optically active direct gap where bound excitons form. Due to band folding in the supercells, it is much more challenging to extract ZPR effects on non-extremal bands. However, the exact ZPR of the lowest direct gap is likely to differ only slightly from the fundamental one, such that using the fundamental gap ZPR values has still been found to still significantly improve the agreement of optical absorption spectra with experiment.<sup>19</sup>

TABLE I: ZPR data for both the monolayer and bulk phases of h-BN, computed via Monte Carlo sampling of the effects of phonons on the electronic eigenvalues corresponding to the valence band maximum and conduction band minimum. Convergence with respect to the  $q$ -grid is shown.

| Material    | Phase | Functional | $q$ -grid<br>(supercell size) | ZPR<br>(meV) | Error<br>(meV) |
|-------------|-------|------------|-------------------------------|--------------|----------------|
| <b>h-BN</b> | Bulk  | PBE        | $3 \times 3 \times 1$         | -195         | 37             |
|             |       |            | $6 \times 6 \times 2$         | -262         | 8              |
|             | 1L    | PBE        | $6 \times 6 \times 1$         | -381         | 48             |
|             |       |            | $9 \times 9 \times 1$         | -383         | 29             |

## D. Atomic Geometries

The atomic structures of the primitive unit cell, used also for the construction of the supercells, as well as the high-symmetry points of the band structures employed in this work, are taken from Refs. 8 and 9, and references therein. They are provided here in the VASP POSCAR format.

### Black phosphorus (bP)

From Ref. 31:

#### Bulk bP

P

1.0

3.3132998943 0.0000000000 0.0000000000  
0.0000000000 10.4729995728 0.0000000000  
0.0000000000 0.0000000000 4.3740000725

P

8

Cartesian

0.0000000000 1.082908150 0.352544410  
0.0000000000 9.390091501 4.021455565  
0.0000000000 4.153591714 2.539544544  
0.0000000000 6.319407858 1.834455659  
1.656649947 6.319407858 0.352544410  
1.656649947 4.153591714 4.021455565  
1.656649947 9.390091501 2.539544544  
1.656649947 1.082908150 1.834455659

#### Monolayer bP

P

1.0

3.3149049282 0.0000000000 0.0000000000  
0.0000000000 4.4248895645 0.0000000000  
0.0000000000 0.0000000000 20.0

P

4

Cartesian

0.0000000000 2.575827533 2.143897536  
0.0000000000 1.849062296 0.0000000000  
1.657452464 0.363382520 0.0000000000  
1.657452464 4.061507078 2.143897536

High-symmetry points for the band structures:

$\Gamma = (0.0, 0.0, 0.0),$

$X = (1/2, 0.0, 0.0),$

$S = (1/2, 1/2, 0.0),$

$Y = (0.0, 1/2, 0.0).$

## MoS<sub>2</sub>

From Ref. 32:

### Bulk MoS<sub>2</sub>

Mo S2

1.0

3.1610000134 0.0000000000 0.0000000000  
-1.5805000067 2.7375063129 0.0000000000  
0.0000000000 0.0000000000 12.2950000763

Mo S

2 4

Cartesian

0.0000000000 1.825004263 3.073750019  
1.580499912 0.912502050 9.221250057  
0.0000000000 1.825004263 7.715112519  
1.580499912 0.912502050 4.579887558  
1.580499912 0.912502050 1.567612480  
0.0000000000 1.825004263 10.727387596

### Monolayer MoS<sub>2</sub>

Mo S2

1.0

3.1610000134 0.0000000000 0.0000000000  
-1.5805000067 2.7375063129 0.0000000000  
0.0000000000 0.0000000000 28.0

Mo S

1 2

Cartesian

0.0000000000 1.825004263 3.073750019  
1.580499912 0.912502050 4.579887558  
1.580499912 0.912502050 1.567612480

High-symmetry points for the band structures:

$\Gamma = (0.0, 0.0, 0.0)$ ,

$K = (1/3, 1/3, 0.0)$ ,

$M = (1/2, 0.0, 0.0)$ .

## h-BN

From Ref. 33.

### Bulk h-BN

BN

1.0

2.4982399940 0.0000000000 0.0000000000  
-1.2491199970 2.1635392996 0.0000000000  
0.0000000000 0.0000000000 6.6357002258

B N

2 2

Cartesian

0.0000000000 0.0000000000 3.317850113  
0.0000000000 1.442359576 0.0000000000  
0.0000000000 0.0000000000 0.0000000000  
0.0000000000 1.442359576 3.31785011

### Monolayer h-BN

BN

1.0

2.4982399940 0.0000000000 0.0000000000  
-1.2491199970 2.1635392996 0.0000000000  
0.0000000000 0.0000000000 25.0

B N

1 1

Cartesian

0.0000000000 0.0000000000 3.317850113  
0.0000000000 1.442359576 3.31785011

High-symmetry points for the band structures:

$\Gamma = (0.0, 0.0, 0.0),$

$K = (1/3, 1/3, 0.0),$

$M = (1/2, 0.0, 0.0).$

### III. PARAMETERS AND NUMERICAL DATA

The following tables summarize the parameters employed in the tuning procedure and subsequent calculations. We also summarize the results obtained with these parameters.

TABLE II: Parameters employed in the SRSB calculations: Supercell size and type for Wannier-optimal tuning; Brillouin zone sampling for primitive cells; average inverse macroscopic dielectric constant ( $\epsilon_\infty^{-1}$ ); and tuned SRSB parameters with the semiempirical (SE) approach ( $\alpha_{\text{SE}}^*, \gamma_{\text{SE}}^*$ ) [Refs. 8 and 9] and the WOT method ( $\alpha_{\text{WOT}}^*, \gamma_{\text{WOT}}^*$ ).

| Material               | Phase | Supercell size         | Supercell type | $k$ -grid               | $\epsilon_\infty^{-1}$ | $\alpha_{\text{SE}}^*$ | $\gamma_{\text{SE}}^*(\text{\AA}^{-1})$ | $\alpha_{\text{WOT}}^*$ | $\gamma_{\text{WOT}}^*(\text{\AA}^{-1})$ |
|------------------------|-------|------------------------|----------------|-------------------------|------------------------|------------------------|-----------------------------------------|-------------------------|------------------------------------------|
| <b>bP</b>              | Bulk  | $5 \times 4 \times 2$  | Orthorhombic   | $8 \times 8 \times 4$   | 0.095                  | 0.170                  | 0.035                                   | 0.152                   | 0.027                                    |
|                        | 1L    | $5 \times 4 \times 1$  | Orthorhombic   | $15 \times 15 \times 1$ | 1.0                    |                        |                                         |                         |                                          |
| <b>MoS<sub>2</sub></b> | Bulk  | $4 \times 4 \times 2$  | Hexagonal      | $12 \times 12 \times 4$ | 0.085                  | 0.107                  | 0.038                                   | 0.126                   | 0.030                                    |
|                        | 1L    | $5 \times 5 \times 1$  | Hexagonal      | $18 \times 18 \times 1$ | 1.0                    |                        |                                         |                         |                                          |
| <b>h-BN</b>            | Bulk  | $5 \times 3 \times 2$  | Orthorhombic   | $12 \times 12 \times 4$ | 0.25                   | 0.201                  | 0.072                                   | 0.341                   | 0.085                                    |
|                        | 1L    | $10 \times 6 \times 1$ | Orthorhombic   | $18 \times 18 \times 1$ | 1.0                    |                        |                                         |                         |                                          |

- 
- \* Corresponding authors: maria.camarasa-gomez@weizmann.ac.il, ashwin@engin.umass.edu, leeor.kronik@weizmann.ac.il
- <sup>1</sup> G. Kresse and J. Furthmüller, *Comput. Mater. Sci.* **6**, 15 (1996).
  - <sup>2</sup> G. Kresse and J. Furthmüller, *Phys. Rev. B* **54**, 11169 (1996).
  - <sup>3</sup> P. E. Blöchl, *Phys. Rev. B* **50**, 17953 (1994).
  - <sup>4</sup> G. Kresse and D. Joubert, *Phys. Rev. B* **59**, 1758 (1999).
  - <sup>5</sup> D. M. Ceperley and B. J. Alder, *Phys. Rev. Lett.* **45**, 566 (1980).
  - <sup>6</sup> J. P. Perdew and A. Zunger, *Phys. Rev. B* **23**, 5048 (1981).
  - <sup>7</sup> D. Wing, G. Ohad, J. B. Haber, M. R. Filip, S. E. Gant, J. B. Neaton, and L. Kronik, *PNAS* **118**, e2104556118 (2021).
  - <sup>8</sup> A. Ramasubramaniam, D. Wing, and L. Kronik, *Phys. Rev. Materials* **3**, 084007 (2019).
  - <sup>9</sup> M. Camarasa-Gómez, A. Ramasubramaniam, J. B. Neaton, and L. Kronik, *Phys. Rev. Mater.* **7**, 104001 (2023).
  - <sup>10</sup> A. A. Mostofi, J. R. Yates, Y.-S. Lee, I. Souza, D. Vanderbilt, and N. Marzari, *Comput. Phys. Commun.* **178**, 685 (2008).
  - <sup>11</sup> M. Gajdoš, K. Hummer, G. Kresse, J. Furthmüller, and F. Bechstedt, *Phys. Rev. B* **73**, 045112 (2006).
  - <sup>12</sup> R. W. Nunes and X. Gonze, *Phys. Rev. B* **63**, 155107 (2001).
  - <sup>13</sup> I. Souza, J. Íñiguez, and D. Vanderbilt, *Phys. Rev. Lett.* **89**, 117602 (2002).
  - <sup>14</sup> M. Leslie and N. J. Gillan, *Journal of Physics C: Solid State Physics* **18**, 973 (1985).
  - <sup>15</sup> G. Makov and M. C. Payne, *Phys. Rev. B* **51**, 4014 (1995).
  - <sup>16</sup> R. Rurali and X. Cartoixa, *Nano Letters* **9**, 975 (2009), pMID: 19206213, <https://doi.org/10.1021/nl802847p>.
  - <sup>17</sup> H.-P. Komsa and A. V. Krashennnikov, *Phys. Rev. B* **86**, 241201 (2012).
  - <sup>18</sup> G. Ohad, D. Wing, S. E. Gant, A. V. Cohen, J. B. Haber, F. Sagredo, M. R. Filip, J. B. Neaton, and L. Kronik, *Phys. Rev. Materials* **6**, 104606 (2022).
  - <sup>19</sup> G. Ohad, S. E. Gant, D. Wing, J. B. Haber, M. Camarasa-Gómez, F. Sagredo, M. R. Filip, J. B. Neaton, and L. Kronik, *Phys. Rev. Mater.* **7**, 123803 (2023).

- <sup>20</sup> A. Laturia, M. L. Van de Put, and W. G. Vandenberghe, npj 2D Materials and Applications **2**, 6 (2018).
- <sup>21</sup> J.-Y. Noh, H. Kim, and Y.-S. Kim, Phys. Rev. B **89**, 205417 (2014).
- <sup>22</sup> P. Giannozzi, S. Baroni, N. Bonini, M. Calandra, R. Car, C. Cavazzoni, Davide Ceresoli, G. L. Chiarotti, M. Cococcioni, I. Dabo, A. D. Corso, S. de Gironcoli, S. Fabris, G. Fratesi, R. Gebauer, U. Gerstmann, C. Gougoussis, Anton Kokalj, M. Lazzeri, L. Martin-Samos, N. Marzari, F. Mauri, R. Mazzarello, Stefano Paolini, A. Pasquarello, L. Paulatto, C. Sbraccia, S. Scandolo, G. Schlauser, A. P. Seitsonen, A. Smogunov, P. Umari, and R. M. Wentzcovitch, J. Phys.: Condens. Matter **21**, 395502 (2009).
- <sup>23</sup> P. Giannozzi and et al., J. Phys.: Condens. Matter **29**, 465901 (2017).
- <sup>24</sup> J. P. Perdew, K. Burke, and M. Ernzerhof, Phys. Rev. Lett. **77**, 3865 (1996).
- <sup>25</sup> D. R. Hamann, Phys. Rev. B **88**, 085117 (2013).
- <sup>26</sup> M. J. van Setten, M. Giantomassi, E. Bousquet, M. J. Verstraete, D. R. Hamann, X. Gonze, and G. M. Rignanese, Comput. Phys. Commun. **226**, 39 (2018).
- <sup>27</sup> B. Monserrat, Phys. Rev. B **93**, 100301 (2016).
- <sup>28</sup> B. Monserrat, J. Phys.: Condens. Matter **30**, 083001 (2018).
- <sup>29</sup> J. H. Lloyd-Williams and B. Monserrat, Phys. Rev. B **92**, 184301 (2015).
- <sup>30</sup> A. Miglio, V. Brousseau-Couture, E. Godbout, G. Antonius, Y.-H. Chan, S. G. Louie, M. Côté, M. Giantomassi, and X. Gonze, NPJ Computational Materials **6**, 167 (2020).
- <sup>31</sup> L. Cartz, S. R. Srinivasa, R. J. Riedner, J. D. Jorgensen, and T. G. Worlton, J. Chem. Phys. **71**, 1718 (1979).
- <sup>32</sup> B. Schönfeld, J. J. Huang, and S. C. Moss, Acta. Crystallogr. B. Struct. Sci. Cryst. Eng. Mater. **39**, 404 (1983).
- <sup>33</sup> A. Brager, Acta Physicochimica (USSR) **7**, 699 (1937).
